# Supplementary material for: The Phase-Coupled Caldeira-Leggett Model: Non-Markovian Open Quantum Dynamics beyond Linear Dissipation
Source: arXiv:2510.25133 ancillary file (2025-10-29)
Supplement: Supplementary file 1 [file sm.pdf]

# Supplementary materials for "The Phase-Coupled Caldeira-Leggett Model: Non-Markovian Open Quantum Dynamics beyond Linear Dissipation"

Ao-Xiang Chang,[1,2] Yu Su,[1] Zi-Fan Zhu,[1] Yao Wang,[1] Rui-Xue Xu,[1] and YiJing Yan[1]

[1]*Hefei National Research Center for Physical Sciences at the Microscale, University of Science and Technology of China, Hefei, Anhui 230026, China*

[2]*Department of Modern Physics, University of Science and Technology of China, Hefei, Anhui 230026, China*

(Dated: October 25, 2025)

These supplementary materials contain (I) Details of Hermite polynomials and generalized normal ordering, (II) Derivation of equations of motion [Eq.(15) of the main text], and (III) Numerical validity of truncation for equations of motion.

## I. HERMITE POLYNOMIALS AS FUNCTION OF DISSIPATON OPERATOR

In this section, we present the detailed derivation of the properties of Hermite polynomials. We consider the case that only one dissipaton involves, that is, $\hat{F} = \hat{f}$. The generalized Wick's theorem reads

$$\mathrm{tr}_{\mathrm{B}}[\mathcal{O}(\hat{f}^n)\hat{f}^{>}\rho_{\mathrm{T}}] = \mathrm{tr}_{\mathrm{B}}[\mathcal{O}(\hat{f}^{n+1})\rho_{\mathrm{T}}] + n\eta\,\mathrm{tr}_{\mathrm{B}}[\mathcal{O}(\hat{f}^{n-1})\rho_{\mathrm{T}}] \tag{S1a}$$

and

$$\mathrm{tr}_{\mathrm{B}}[\mathcal{O}(\hat{f}^n)\hat{f}^{<}\rho_{\mathrm{T}}] = \mathrm{tr}_{\mathrm{B}}[\mathcal{O}(\hat{f}^{n+1})\rho_{\mathrm{T}}] + n\eta^*\mathrm{tr}_{\mathrm{B}}[\mathcal{O}(\hat{f}^{n-1})\rho_{\mathrm{T}}]. \tag{S1b}$$

Here, we only consider the left action case, since the right action one is the same. As some examples, we have (Here, we omit the left action label and the trace outside)

$$\begin{aligned} \hat{f} &= \mathcal{O}(\hat{f}), \\ \hat{f}^2 &= \mathcal{O}(\hat{f})\hat{f} = \mathcal{O}(\hat{f}^2) + \eta, \\ \hat{f}^3 &= \mathcal{O}(\hat{f}^2)\hat{f} + \eta\hat{f} = \mathcal{O}(\hat{f}^3) + 3\eta\hat{f}, \end{aligned} \tag{S2}$$

Define the Hermite polynomials as

$$H_n^{>}(\hat{f}) \equiv \frac{\mathrm{d}^n}{\mathrm{d}z^n} e^{z\hat{f}-\eta z^2/2}\Big|_{z=0}, \tag{S3}$$

for $n = 0, 1, 2, \cdots$. As a result, we can verify that

$$\mathcal{O}(\hat{f}^n) = H_n^{>}(\hat{f}) \quad \text{and} \quad \hat{f}^n = i^{-n}\mathcal{O}[H_n^{>}(i\hat{f})]. \tag{S4}$$

Then we have

$$e^{i\lambda\hat{f}} = \sum_{n=0}^{\infty}\frac{(i\lambda)^n}{n!}\hat{f}^n = \mathcal{O}\sum_{n=0}^{\infty}\frac{\lambda^n}{n!}H_n^{>}(i\hat{f}) = \mathcal{O}e^{i\lambda\hat{f}-\eta\lambda^2/2}. \tag{S5}$$

Consequently,

$$\mathcal{O}(\hat{f}^n)e^{i\lambda\hat{f}^{>}} = e^{-\eta\lambda^2/2}\sum_{m=0}^{\infty}\frac{(i\lambda)^m}{m!}\mathcal{O}(\hat{f}^n)\mathcal{O}(\hat{f}^m)^{>}. \tag{S6}$$

From

$$e^{u\hat{f}-\eta u^2/2}e^{v\hat{f}-\eta v^2/2} = e^{(u+v)\hat{f}-\eta(u^2+v^2)/2} = \mathcal{O}e^{(u+v)\hat{f}+\eta uv} \tag{S7}$$

and

$$e^{u\hat{f}-\eta u^2/2} = \sum_{m=0}^{\infty} \frac{u^m}{m!} H_m^{>}(\hat{f}), \tag{S8}$$

we have

$$H_m^{>}(\hat{f}) H_n^{>}(\hat{f}) = \frac{\partial^{m+n}}{\partial u^m \partial v^n} \mathcal{O} e^{(u+v)\hat{f}+uv\eta} \Big|_{u=v=0} = \frac{\partial^n}{\partial v^n} \mathcal{O}\left[(v\eta + \hat{f})^m e^{v\hat{f}}\right] \Big|_{v=0}. \tag{S9}$$

Noting

$$(v\eta + \hat{f})^m = \sum_{l=0}^{\infty} \frac{1}{l!} \frac{\partial^l}{\partial v^l} (v\eta + \hat{f})^m \Big|_{v=0} v^l = \sum_{l=0}^{m} \binom{m}{l} \eta^l \hat{f}^{m-l} v^l, \tag{S10}$$

we obtain

$$\frac{\partial^l}{\partial v^l} (v\eta + \hat{f})^m \Big|_{v=0} = \begin{cases} 0, & l > m, \\ l! \binom{m}{l} \eta^l \hat{f}^{m-l}, & l \leq m. \end{cases} \tag{S11}$$

As a result,

$$\begin{aligned} \frac{\partial^n}{\partial v^n} \left[(v\eta + \hat{f})^m e^{v\hat{f}}\right] \Big|_{v=0} &= \sum_{l=0}^{n} \binom{n}{l} \frac{\partial^l}{\partial v^l} (v\eta + \hat{f})^m \Big|_{v=0} \frac{\partial^{n-l}}{\partial v^{n-l}} e^{v\hat{f}} \Big|_{v=0} \\ &= \sum_{l=0}^{\min(m,n)} \binom{m}{l} \binom{n}{l} \eta^l l! \hat{f}^{m+n-2l}. \end{aligned} \tag{S12}$$

Go back to Eq. (S9), and we obtain

$$\mathcal{O}(\hat{f}^m) \mathcal{O}(\hat{f}^n) = \sum_{l=0}^{\min(m,n)} \binom{m}{l} \binom{n}{l} \eta^l l! \mathcal{O}(\hat{f}^{m+n-2l}). \tag{S13}$$

By substituting Eq. (S13) into Eq. (S6), we have

$$\mathcal{O}(\hat{f}^n) e^{i\lambda \hat{f}^{>}} = e^{-\frac{\eta\lambda^2}{2}} \sum_{m=0}^{\infty} \sum_{l=0}^{\min(m,n)} \frac{(i\lambda)^m \eta^l}{(m-l)!} \binom{n}{l} \mathcal{O}(\hat{f}^{n+m-2l}). \tag{S14}$$

For the convenience of numerical realization, one may change the summation label into

$$\mathcal{O}(\hat{f}^n) e^{i\lambda \hat{f}^{>}} = e^{-\frac{\eta\lambda^2}{2}} \sum_{k=0}^{\infty} \sum_{m=|n-k|}^{n+k}{}' \frac{(i\lambda)^m \eta^{(m+n-k)/2}}{(m-(m+n-k)/2)!} \binom{n}{(m+n-k)/2} \mathcal{O}(\hat{f}^k). \tag{S15}$$

Here the prime summation is over those $m = k - n \pmod 2$.

## II. DERIVATION OF EQUATIONS OF MOTION [EQ.(15) OF THE MAIN TEXT]

We consider the total Hamiltonian as

$$H_{\mathrm{T}} = H_{\mathrm{S}} + H_{\mathrm{B}} + H_{\mathrm{SB}}, \tag{S16}$$

where $H_{\mathrm{S}}$ is the system Hamiltonian,

$$H_{\mathrm{B}} = \sum_j \frac{\omega_j}{2} (p_j^2 + x_j^2) \tag{S17}$$

is the bath Hamiltonian, and $H_{\rm SB}$ is the system-bath coupling Hamiltonian, taking the form of

$$H_{\rm SB} = \hat{S}\hat{B} = \hat{S}(e^{i\lambda\hat{F}} + e^{-i\lambda\hat{F}}). \tag{S18}$$

Here, $\hat{S}$ is a system operator and $\hat{B}$ is generated by the exponential of the collective bath coordinate $\hat{F} = \sum_j c_j x_j$. After the dissipaton decomposition, $\hat{F} \to \sum_k \hat{f}_k$, we denote

$$\rho_{\mathbf{n}}^{(n)}(t) \equiv \rho_{n_1\cdots n_K}^{(n)}(t) = {\rm tr}_{\rm B}\Big[\mathcal{O}\Big(\prod_{k=1}^{K}\hat{f}_k^{n_k}\Big)\rho_{\rm T}(t)\Big], \tag{S19}$$

with $n = \sum_k n_k$. From the total space Liouville–von Neumann equation,

$$\rho_{\rm T}(t) = -i[H_{\rm T}, \rho_{\rm T}(t)] = -i[H_{\rm S}, \rho_{\rm T}(t)] - i[H_{\rm B}, \rho_{\rm T}(t)] - i[H_{\rm SB}, \rho_{\rm T}(t)], \tag{S20}$$

we derive the equations of motion for $\rho_{\mathbf{n}}^{(n)}(t)$ term by term. We denote

$$\dot{\rho}_{\mathbf{n}}^{(n)}(t) = {\rm tr}_{\rm B}\Big[\mathcal{O}\Big(\prod_{k=1}^{K}\hat{f}_k^{n_k}\Big)\dot{\rho}_{\rm T}(t)\Big] = -i{\rm tr}_{\rm B}\Big\{\mathcal{O}\Big(\prod_{k=1}^{K}\hat{f}_k^{n_k}\Big)[H_{\rm S} + H_{\rm B} + H_{\rm SB}, \rho_{\rm T}(t)]\Big\}. \tag{S21}$$

(I) The system Hamiltonian term:

$$-i{\rm tr}_{\rm B}\Big\{\mathcal{O}\Big(\prod_{k=1}^{K}\hat{f}_k^{n_k}\Big)[H_{\rm S}, \rho_{\rm T}(t)]\Big\} = -i[H_{\rm S}, \rho_{\mathbf{n}}^{(n)}(t)]. \tag{S22}$$

(II) The bath Hamiltonian term:

$$-i{\rm tr}_{\rm B}\Big\{\mathcal{O}\Big(\prod_{k=1}^{K}\hat{f}_k^{n_k}\Big)[H_{\rm B}, \rho_{\rm T}(t)]\Big\} = -i{\rm tr}_{\rm B}\Big\{\Big[\mathcal{O}\Big(\prod_{k=1}^{K}\hat{f}_k^{n_k}\Big), H_{\rm B}\Big]\rho_{\rm T}(t)\Big\} = -\sum_k n_k\gamma_k\rho_{\mathbf{n}}^{(n)}(t). \tag{S23}$$

Here, we have used the generalized diffusion equation, [Eq.(7) of the main text],

$$-i{\rm tr}_{\rm B}\Big\{\big[\mathcal{O}(\hat{f}_k^{n_k}), H_{\rm B}\big]\rho_{\rm T}(t)\Big\} = {\rm tr}_{\rm B}\big[\mathcal{O}(\dot{\hat{f}}_k^{n_k})\rho_{\rm T}(t)\big] = -n_k\gamma_k{\rm tr}_{\rm B}\big[\mathcal{O}(\hat{f}_k^{n_k})\rho_{\rm T}(t)\big]. \tag{S24}$$

(III) The system-bath coupling Hamiltonian term: Using Eq. (S14), we firstly consider

$$\begin{aligned}
-i{\rm tr}_{\rm B}\Big[\mathcal{O}\Big(\prod_{k=1}^{K}\hat{f}_k^{n_k}\Big)\hat{S}e^{i\lambda\hat{F}}\rho_{\rm T}(t)\Big] &= -i\hat{S}{\rm tr}_{\rm B}\Big[\mathcal{O}\Big(\prod_{k=1}^{K}\hat{f}_k^{n_k}\Big)e^{i\lambda\hat{F}}\rho_{\rm T}(t)\Big] \\
&= -i\hat{S}{\rm tr}_{\rm B}\Big\{\mathcal{O}\Big[\prod_k e^{-\eta_k\lambda^2/2}\sum_{m_k=0}^{\infty}\sum_{l_k=0}^{\min(m_k,n_k)}\frac{(i\lambda)^{m_k}\eta_k^{l_k}}{(m_k-l_k)!}\binom{n_k}{l_k}\hat{f}_k^{n_k+m_k-2l_k}\Big]\rho_{\rm T}(t)\Big\} \\
&= -ig\hat{S}{\sum_{\mathbf{m},\mathbf{l}}}'(i\lambda)^m\prod_k\frac{\eta_k^{l_k}}{(m_k-l_k)!}\binom{n_k}{l_k}\rho_{\mathbf{n}+\mathbf{m}-2\mathbf{l}}^{(n+m-2l)},
\end{aligned} \tag{S25}$$

where we denote

$$g \equiv \prod_k e^{-\eta_k\lambda^2/2} = e^{-\langle\hat{F}^2\rangle_{\rm B}\lambda^2/2} \tag{S26}$$

and the prime summation

$${\sum_{\mathbf{m},\mathbf{l}}}' \equiv \sum_{m_1=0}^{\infty}\cdots\sum_{m_K=0}^{\infty}\sum_{l_1=0}^{\min(m_1,n_1)}\cdots\sum_{l_K=0}^{\min(m_K,n_K)}. \tag{S27}$$

Then the other three terms can be derived in a similar way. Finally, we arrive at the equations of motion,

$$\begin{aligned}
\dot{\rho}_{\mathbf{n}}^{(n)} = &-i[H_{\rm S}, \rho_{\mathbf{n}}^{(n)}] - \sum_k n_k\gamma_k\rho_{\mathbf{n}}^{(n)} - ig{\sum_{\mathbf{m},\mathbf{l}}}'[(i\lambda)^m - (-i\lambda)^m]\prod_k\frac{\eta_k^{l_k}}{(m_k-l_k)!}\binom{n_k}{l_k}\hat{S}\rho_{\mathbf{n}+\mathbf{m}-2\mathbf{l}}^{(n+m-2l)} \\
&+ ig{\sum_{\mathbf{m},\mathbf{l}}}'[(i\lambda)^m - (-i\lambda)^m]\prod_k\frac{\eta_{\bar{k}}^{*l_k}}{(m_k-l_k)!}\binom{n_k}{l_k}\rho_{\mathbf{n}+\mathbf{m}-2\mathbf{l}}^{(n+m-2l)}\hat{S}.
\end{aligned} \tag{S28}$$

This is Eq. (15) in the main text, the central result of our work.

## III. NUMERICAL VALIDITY OF TRUNCATION FOR EQ. (15)

In this section, we present the convergence of time evolution of Eq. (15) with increasing the truncation order $L$. We consider the same model as in Fig. 2 of the main text. The results are shown in Fig. S1. It is seen that the results converge quickly with increasing $L$. The results with $L = 4$ and $L = 6$ are almost indistinguishable.

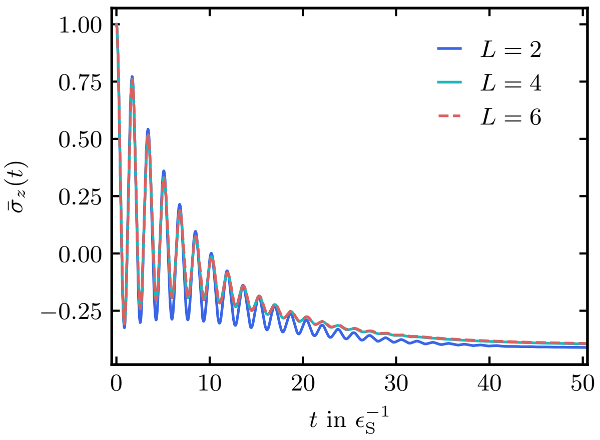


FIG. S1. Time evolution of $\bar{\sigma}_z(t) = \langle 0|\rho_{\mathrm{S}}(t)|0\rangle - \langle 1|\rho_{\mathrm{S}}(t)|1\rangle$ under different truncation order $L$. The parameters are the same as those in Fig. 2 of the main text.
